# Supplementary material for: Joint Image and Depth Estimation with Mask-Based Lensless Cameras
Source: arXiv:1910.02526 source file (2020-06-19)
Supplement: Supplementary file 1 [file supp.tex]

\subsection{Reconstruction of a Single Plane}
% \subsection{Limits of depth estimation}
To understand various parameters of our method and their effect on depth estimation, we perform a simple simulation experiment in which the scene consists of a single plane and our goal is to recover the correct depth accurately. In other words, the depth map is parameterized by a scalar $\balpha$ instead of a matrix of the same size as intensity $\mathbf{l}$. The estimation of the single depth parameter does not involve the regularization, so we solve \eqref{eq:final_optimization} via alternating minimization using Algorithm~\ref{alg:l2_algorithm} without the regularization term. We test the performance of our optimization program using a USAF target image placed at three different depths in the scene: $[10cm, 1m, 10m]$. We test two different initialization schemes for comparison. (1) Initial value of $\balpha$ is selected to set depth at 1km (i.e., $\balpha\approx 1$ for all the experiments). (2) We choose a depth plane from 10 candidate depths that were uniformly sampled in $\alpha$ to get effective depth range from 9cm to 1km; for a given measurement we selected $\balpha$ that provided smallest loss function in \eqref{eq:final_optimization}. To separate the effect of image estimate and depth estimate, we tested two cases: one in which image intensity is an optimization variable and updated iteratively and the other one where the image intensity is fixed to its original value. Since the problem in \eqref{eq:final_optimization} is nonconvex in $\balpha$ even if we fix the value of intensity $\mathbf{l}$, there is no guarantee we can estimate the correct value of $\balpha$.

\begin{figure}[thb!]
    \captionsetup[subfigure]{position=b}
    \centering
    \begin{subfigure}[t]{0.49\linewidth}
    \includegraphics[width=1\linewidth]{figures/inf_annotated.png}
    \caption{Convergence of estimates; initial depth at 1km. We annotate the starting depth and converged depth in the plot.
    % Dotted lines stand for known image and solid lines stand for unknown image.
    }
    \end{subfigure}
    \begin{subfigure}[t]{0.49\linewidth}
    \includegraphics[width=1\linewidth]{figures/swap_annotated.png}
    \caption{Convergence of estimates; initial depth selected from 10 candidate planes. We annotate the starting depth and converged depth in the plot.
    % Dotted lines stand for known image and solid lines stand for unknown image.
    }
    \end{subfigure}
    
    \begin{subfigure}[t]{0.24\linewidth}
    \includegraphics[width=1\linewidth]{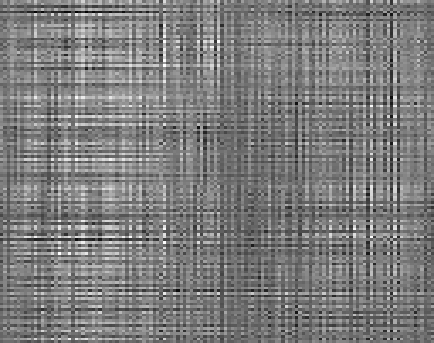}
    \caption{Initial depth 1km. Image intensity unknown}
    \end{subfigure}
    \begin{subfigure}[t]{0.24\linewidth}
    \includegraphics[width=1\linewidth]{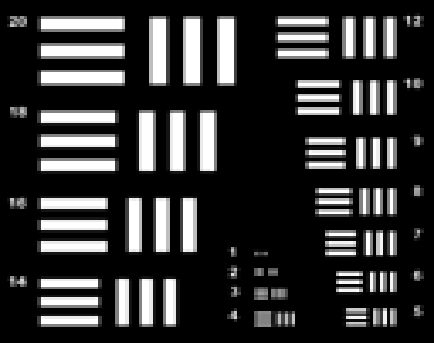}
    \caption{Initial depth 1km. Image intensity known}
    \end{subfigure}
    \begin{subfigure}[t]{0.24\linewidth}
    \includegraphics[width=1\linewidth]{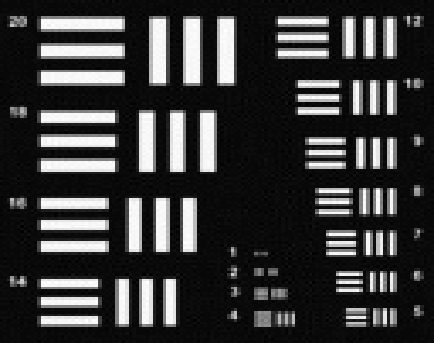}
    \caption{Initial depth selected from 10 planes. Image intensity unknown}
    \end{subfigure}
    \begin{subfigure}[t]{0.24\linewidth}
    \includegraphics[width=1\linewidth]{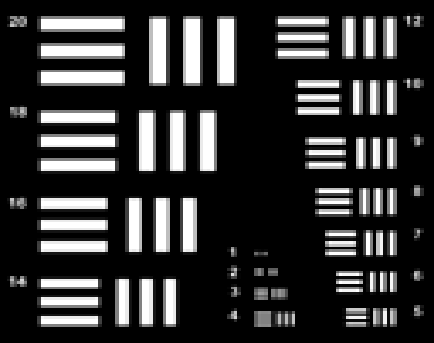}
    \caption{Initial depth selected from 10 planes. Image intensity known}
    \end{subfigure}
    \caption{Recovery of a single depth parameter. USAF target is tested at three different depths with two different types of  initialization. (a) Initial depth is set to 1km. (b) Initial depth is selected out of 10 candidate planes. (a), (b) Reconstruction loss plotted against the depth estimate at every iteration of the algorithm. If the algorithm estimates correct image intensity and depth, the plot should converge to the true depth with a small loss function value. Solid lines correspond to the case when we jointly estimate image intensity and depth. Dashed lines correspond to the case when image intensities are known. (c)--(d) Reconstructed images when the original scene is 10cm away, under different choice of initial depth and unknown/known image intensities. The loss function values for all the experiment refer to the squared error between approximation measurements and captured sensor measurements.}
    \label{fig:loss_single_depth_curve}
\end{figure}

We report the results for 12 experiments (image at three different depths with two different initialization and known or unknown image intensity) in Figure~\ref{fig:loss_single_depth_curve}. Figures~\ref{fig:loss_single_depth_curve}(a) and (b) plot the loss function at the estimated depth at every iteration of the refinement step in Algorithm~\ref{alg:l2_algorithm} for the cases when the initial depth is set to 1km and when the initial depth is selected out of 10 candidate depths. From the curves in Figure~\ref{fig:loss_single_depth_curve}(a), we observe that we can estimate the depth accurately in all three cases when the image intensities are known (dashed lines). If we jointly estimate the depth and image intensities, the initial value of depth plays a critical role (solid lines). We observe that the intensity and depth are recovered correctly for the scene at 1m and 10m but the algorithm fails to recover correct depth for the scene at 10cm. This is mainly because the initial value of $\balpha$ is very far from the true value and the algorithm is more likely to get stuck in a local minimum. Figure~\ref{fig:loss_single_depth_curve}(c) shows the reconstructed image when the original scene is at 10cm away, initial depth is set to 1km, and we estimate image intensity and depth by solving \eqref{eq:final_optimization}. On the other hand, when we pick initial depth close to the true depth (out of 10 candidates, using a greedy approach), as shown in Figure~\ref{fig:loss_single_depth_curve}(b), the algorithm converges to the true depth and recover the correct image intensities as well.

% NUMBER OF SENSOR PIXELS

\begin{figure*}
\centering
    \begin{subfigure}{\figwidth}
    \caption*{Original}
    \includegraphics[width=1\linewidth]{figures_results/sword2_scene_image.png}
    \caption*{Image PSNR:}
    \includegraphics[width=1\linewidth]{figures_results/sword2_scene_depth.png}
        \caption*{Depth RMSE:}
    \end{subfigure}
    \begin{subfigure}{\figwidth}
    \caption*{$256\times256$} 
    \includegraphics[width=1\linewidth]{figures_results/sword2_sensor_256_image.png}
    \caption*{16.51dB} 
    \includegraphics[width=1\linewidth]{figures_results/sword2_sensor_256_depth.png}
        \caption*{74.76mm} 
    \end{subfigure}
        \begin{subfigure}{\figwidth}
    \caption*{$512\times512$} 
    \includegraphics[width=1\linewidth]{figures_results/sword2_sensor_512_image.png}
    \caption*{22.27dB} 
    \includegraphics[width=1\linewidth]{figures_results/sword2_sensor_512_depth.png}
        \caption*{34.39mm} 
    \end{subfigure}
        \begin{subfigure}{\figwidth}
    \caption*{$1024\times1024$} 
    \includegraphics[width=1\linewidth]{figures_results/sword2_sensor_1024_image.png}
    \caption*{27.79dB} 
    \includegraphics[width=1\linewidth]{figures_results/sword2_sensor_1024_depth.png}
        \caption*{11.17mm} 
    \end{subfigure}
    ~~~
   \begin{subfigure}{\figwidth}
   \caption*{Original}
    \includegraphics[width=1\linewidth]{figures_results/playtable_scene_image.png}
    \caption*{Image PSNR:}
    \includegraphics[width=1\linewidth]{figures_results/playtable_scene_depth.png}
        \caption*{Depth RMSE:}
    \end{subfigure}
    \begin{subfigure}{\figwidth}
    \caption*{$256\times256$}
    \includegraphics[width=1\linewidth]{figures_results/playtable_sensor_256_image.png}
    \caption*{25.55dB} 
    \includegraphics[width=1\linewidth]{figures_results/playtable_sensor_256_depth.png}
        \caption*{248.78mm} 
    \end{subfigure}
        \begin{subfigure}{\figwidth}
        \caption*{$512\times512$}
    \includegraphics[width=1\linewidth]{figures_results/playtable_sensor_512_image.png}
    \caption*{31.05dB} 
    \includegraphics[width=1\linewidth]{figures_results/playtable_sensor_512_depth.png}
        \caption*{147.68mm} 
    \end{subfigure}
        \begin{subfigure}{\figwidth}
        \caption*{$1024\times1024$}
    \includegraphics[width=1\linewidth]{figures_results/playtable_sensor_1024_image.png}
    \caption*{32.79dB} 
    \includegraphics[width=1\linewidth]{figures_results/playtable_sensor_1024_depth.png}
        \caption*{107.04mm} 
    \end{subfigure}
    \centering
    \begin{subfigure}{\figwidth}
    \caption*{Original}
    \includegraphics[width=1\linewidth]{figures_results/whiteboard_scene_image.png}
    \caption*{Image PSNR:}
    \includegraphics[width=1\linewidth]{figures_results/whiteboard_scene_depth.png}
        \caption*{Depth RMSE:}
    \end{subfigure}
    \begin{subfigure}{\figwidth}
    \caption*{$256\times256$} 
    \includegraphics[width=1\linewidth]{figures_results/whiteboard_sensor_256_image.png}
    \caption*{21.70dB}
    \includegraphics[width=1\linewidth]{figures_results/whiteboard_sensor_256_depth.png}
        \caption*{177.80mm} 
    \end{subfigure}
        \begin{subfigure}{\figwidth}
    \caption*{$512\times512$} 
    \includegraphics[width=1\linewidth]{figures_results/whiteboard_sensor_512_image.png}
    \caption*{28.64dB}
    \includegraphics[width=1\linewidth]{figures_results/whiteboard_sensor_512_depth.png}
        \caption*{128.72mm} 
    \end{subfigure}
        \begin{subfigure}{\figwidth}
    \caption*{$1024\times1024$} 
    \includegraphics[width=1\linewidth]{figures_results/whiteboard_sensor_1024_image.png}
    \caption*{30.47dB}
    \includegraphics[width=1\linewidth]{figures_results/whiteboard_sensor_1024_depth.png}
        \caption*{160.50mm} 
    \end{subfigure}
    ~~~
    \begin{subfigure}{\figwidth}
    \caption*{Original} \includegraphics[width=1\linewidth]{figures_results/playroom_scene_image.png}
    \caption*{Image PSNR:}
    \includegraphics[width=1\linewidth]{figures_results/playroom_scene_depth.png}
        \caption*{Depth RMSE:}
    \end{subfigure}
    \begin{subfigure}{\figwidth}
    \caption*{$256\times256$} \includegraphics[width=1\linewidth]{figures_results/playroom_sensor_256_image.png}
    \caption*{27.48dB}
    \includegraphics[width=1\linewidth]{figures_results/playroom_sensor_256_depth.png}
        \caption*{182.45mm} 
    \end{subfigure}
        \begin{subfigure}{\figwidth}
    \caption*{$512\times512$} \includegraphics[width=1\linewidth]{figures_results/playroom_sensor_512_image.png}
    \caption*{32.99dB}
    \includegraphics[width=1\linewidth]{figures_results/playroom_sensor_512_depth.png}
        \caption*{129.04mm} 
    \end{subfigure}
        \begin{subfigure}{\figwidth}
    \caption*{$1024\times1024$} \includegraphics[width=1\linewidth]{figures_results/playroom_sensor_1024_image.png}
    \caption*{35.48dB}
    \includegraphics[width=1\linewidth]{figures_results/playroom_sensor_1024_depth.png}
        \caption*{81.89mm} 
    \end{subfigure}

    \begin{subfigure}{\figwidth}
    \includegraphics[width=1\linewidth]{figures_results/moebius_scene_image.png}
    \caption*{Image PSNR:}
    \includegraphics[width=1\linewidth]{figures_results/moebius_scene_depth.png}
        \caption*{Depth RMSE:}
    \end{subfigure}
    \begin{subfigure}{\figwidth}
    \includegraphics[width=1\linewidth]{figures_results/moebius_sensor_256_image.png}
    \caption*{23.58dB}
    \includegraphics[width=1\linewidth]{figures_results/moebius_sensor_256_depth.png}
        \caption*{41.84mm} 
    \end{subfigure}
        \begin{subfigure}{\figwidth}
    \includegraphics[width=1\linewidth]{figures_results/moebius_sensor_512_image.png}
    \caption*{29.64dB}
    \includegraphics[width=1\linewidth]{figures_results/moebius_sensor_512_depth.png}
        \caption*{16.19mm} 
    \end{subfigure}
        \begin{subfigure}{\figwidth}
    \includegraphics[width=1\linewidth]{figures_results/moebius_sensor_1024_image.png}
    \caption*{31.99dB}
    \includegraphics[width=1\linewidth]{figures_results/moebius_sensor_1024_depth.png}
        \caption*{8.12mm} 
    \end{subfigure}
    ~~~
    \begin{subfigure}{\figwidth}
    \includegraphics[width=1\linewidth]{figures_results/book_scene_image.png}
    \caption*{Image PSNR:}
    \includegraphics[width=1\linewidth]{figures_results/book_scene_depth.png}
        \caption*{Depth RMSE:}
    \end{subfigure}
    \begin{subfigure}{\figwidth}
    \includegraphics[width=1\linewidth]{figures_results/book_sensor_256_image.png}
    \caption*{24.63dB}
    \includegraphics[width=1\linewidth]{figures_results/book_sensor_256_depth.png}
        \caption*{43.75mm} 
    \end{subfigure}
        \begin{subfigure}{\figwidth}
    \includegraphics[width=1\linewidth]{figures_results/book_sensor_512_image.png}
    \caption*{31.14dB}
    \includegraphics[width=1\linewidth]{figures_results/book_sensor_512_depth.png}
        \caption*{19.72mm} 
    \end{subfigure}
        \begin{subfigure}{\figwidth}
    \includegraphics[width=1\linewidth]{figures_results/book_sensor_1024_image.png}
    \caption*{33.32dB}
    \includegraphics[width=1\linewidth]{figures_results/book_sensor_1024_depth.png}
        \caption*{13.55mm} 
    \end{subfigure}

      \begin{subfigure}{\figwidth}
    % \caption*{Original}
    \includegraphics[width=1\linewidth]{figures_results/cones_scene_image.png}
    \caption*{Image PSNR:}
    \includegraphics[width=1\linewidth]{figures_results/cones_scene_depth.png}
        \caption*{Depth RMSE:}
    \end{subfigure}
    \begin{subfigure}{\figwidth}
    % \caption*{$256\times256$}
    \includegraphics[width=1\linewidth]{figures_results/cones_sensor_256_image.png}
    \caption*{26.85dB} 
    \includegraphics[width=1\linewidth]{figures_results/cones_sensor_256_depth.png}
        \caption*{56.59mm} 
    \end{subfigure}
        \begin{subfigure}{\figwidth}
        % \caption*{$512\times512$}
    \includegraphics[width=1\linewidth]{figures_results/cones_sensor_512_image.png}
    \caption*{32.83dB} 
    \includegraphics[width=1\linewidth]{figures_results/cones_sensor_512_depth.png}
        \caption*{28.70mm} 
    \end{subfigure}
        \begin{subfigure}{\figwidth}
        % \caption*{$1024\times1024$}
    \includegraphics[width=1\linewidth]{figures_results/cones_sensor_1024_image.png}
    \caption*{35.29dB} 
    \includegraphics[width=1\linewidth]{figures_results/cones_sensor_1024_depth.png}
        \caption*{11.02mm} 
    \end{subfigure}
    ~~~
        \begin{subfigure}{\figwidth}
    \includegraphics[width=1\linewidth]{figures_results/corner_scene_image.png}
    \caption*{Image PSNR:}
    \includegraphics[width=1\linewidth]{figures_results/corner_scene_depth.png}
        \caption*{Depth RMSE:}
    \end{subfigure}
    \begin{subfigure}{\figwidth}
    \includegraphics[width=1\linewidth]{figures_results/corner_sensor_256_image.png}
    \caption*{29.82dB} 
    \includegraphics[width=1\linewidth]{figures_results/corner_sensor_256_depth.png}
        \caption*{439.66mm} 
    \end{subfigure}
        \begin{subfigure}{\figwidth}
    \includegraphics[width=1\linewidth]{figures_results/corner_sensor_512_image.png}
    \caption*{34.15dB} 
    \includegraphics[width=1\linewidth]{figures_results/corner_sensor_512_depth.png}
        \caption*{282.61mm} 
    \end{subfigure}
        \begin{subfigure}{\figwidth}
    \includegraphics[width=1\linewidth]{figures_results/corner_sensor_1024_image.png}
    \caption*{35.69dB} 
    \includegraphics[width=1\linewidth]{figures_results/corner_sensor_1024_depth.png}
        \caption*{194.91mm} 
    \end{subfigure}

    \caption{Results for reconstruction from measurements with different numbers of pixels. The size of each sensor pixel is fixed as 50$\mu$m. }
    \label{fig:number_of_pixels_example_supp}
\end{figure*}

\subsection{Number of Sensor Measurements}
In this experiment, we evaluate the performance of our algorithm as we increase/decrease the number of sensor measurements. The depth estimation problem we are solving is highly ill-posed because of the existence of nontrivial null space of the system matrix and nonlinear dependence of measurements on the depth parameters. 
Adding more measurements helps to improve the solution of the system by adding more constraints on the feasible solutions. 

We perform experiments with different numbers of sensor pixels while the size of each pixel is fixed as 50$\mu$m. We do not add any noise in these experiments to avoid randomness that potentially affects comparison. As we increase or decrease the number of pixels, it is equivalent to increasing or decreasing the sensor area. Therefore, when we increase the number of sensor pixels (equivalently, sensor area), the baseline of the sensor is also increased, which helps us in resolving the depth more accurately. The results are presented in Figure~\ref{fig:number_of_pixels_example_supp} for sensors of size $256\times 256$, $512\times 512$, and $1024\times 1024$. We observe that the quality of both image and depth improves as we use more sensor pixels for measurements.

% NOISE LEVELS
\begin{figure*}
    \centering
    \begin{subfigure}{\figwidth}
    \caption*{Original}
    \includegraphics[width=1\linewidth]{figures_results/whiteboard_scene_image.png}
    \caption*{Image PSNR:}
    \includegraphics[width=1\linewidth]{figures_results/whiteboard_scene_depth.png}
        \caption*{Depth RMSE:}
    \end{subfigure}
        \begin{subfigure}{\figwidth}
    \caption*{20dB} 
    \includegraphics[width=1\linewidth]{figures_results/whiteboard_SNR_20_repeat_ind_1_image.png}
    \caption*{5.58dB}
    \includegraphics[width=1\linewidth]{figures_results/whiteboard_SNR_20_repeat_ind_1_depth.png}
        \caption*{214.12mm} 
    \end{subfigure}
        \begin{subfigure}{\figwidth}
    \caption*{30dB} 
    \includegraphics[width=1\linewidth]{figures_results/whiteboard_SNR_30_repeat_ind_1_image.png}
    \caption*{15.66dB}
    \includegraphics[width=1\linewidth]{figures_results/whiteboard_SNR_30_repeat_ind_1_depth.png}
        \caption*{137.14mm} 
    \end{subfigure}
        \begin{subfigure}{\figwidth}
    \caption*{40dB} 
    \includegraphics[width=1\linewidth]{figures_results/whiteboard_SNR_40_repeat_ind_1_image.png}
    \caption*{24.24dB}
    \includegraphics[width=1\linewidth]{figures_results/whiteboard_SNR_40_repeat_ind_1_depth.png}
        \caption*{130.95mm} 
    \end{subfigure}
    ~~~
        \begin{subfigure}{\figwidth}
   \caption*{Original }  \includegraphics[width=1\linewidth]{figures_results/playroom_scene_image.png}
    \caption*{Image PSNR:}
    \includegraphics[width=1\linewidth]{figures_results/playroom_scene_depth.png}
        \caption*{Depth RMSE:}
    \end{subfigure}
        \begin{subfigure}{\figwidth}
    \caption*{20dB} \includegraphics[width=1\linewidth]{figures_results/playroom_SNR_20_repeat_ind_1_image.png}
    \caption*{5.09dB}
    \includegraphics[width=1\linewidth]{figures_results/playroom_SNR_20_repeat_ind_1_depth.png}
        \caption*{397.02mm} 
    \end{subfigure}
        \begin{subfigure}{\figwidth}
    \caption*{30dB} \includegraphics[width=1\linewidth]{figures_results/playroom_SNR_30_repeat_ind_1_image.png}
    \caption*{15.56dB}
    \includegraphics[width=1\linewidth]{figures_results/playroom_SNR_30_repeat_ind_1_depth.png}
        \caption*{142.37mm} 
    \end{subfigure}
        \begin{subfigure}{\figwidth}
    \caption*{40dB} \includegraphics[width=1\linewidth]{figures_results/playroom_SNR_40_repeat_ind_1_image.png}
    \caption*{25.52dB}
    \includegraphics[width=1\linewidth]{figures_results/playroom_SNR_40_repeat_ind_1_depth.png}
        \caption*{126.78mm} 
    \end{subfigure}
    
         \begin{subfigure}{\figwidth}
    \includegraphics[width=1\linewidth]{figures_results/moebius_scene_image.png}
    \caption*{Image PSNR:}
    \includegraphics[width=1\linewidth]{figures_results/moebius_scene_depth.png}
        \caption*{Depth RMSE:}
    \end{subfigure}
        \begin{subfigure}{\figwidth}
    \includegraphics[width=1\linewidth]{figures_results/moebius_SNR_20_repeat_ind_1_image.png}
    \caption*{4.32dB}
    \includegraphics[width=1\linewidth]{figures_results/moebius_SNR_20_repeat_ind_1_depth.png}
        \caption*{52.57mm} 
    \end{subfigure}
        \begin{subfigure}{\figwidth}
    \includegraphics[width=1\linewidth]{figures_results/moebius_SNR_30_repeat_ind_1_image.png}
    \caption*{14.52dB}
    \includegraphics[width=1\linewidth]{figures_results/moebius_SNR_30_repeat_ind_1_depth.png}
        \caption*{22.25mm} 
    \end{subfigure}
        \begin{subfigure}{\figwidth}
    \includegraphics[width=1\linewidth]{figures_results/moebius_SNR_40_repeat_ind_1_image.png}
    \caption*{23.66dB}
    \includegraphics[width=1\linewidth]{figures_results/moebius_SNR_40_repeat_ind_1_depth.png}
        \caption*{17.06mm} 
    \end{subfigure}
    ~~~
            \begin{subfigure}{\figwidth}
    \includegraphics[width=1\linewidth]{figures_results/book_scene_image.png}
    \caption*{Image PSNR:}
    \includegraphics[width=1\linewidth]{figures_results/book_scene_depth.png}
        \caption*{Depth RMSE:}
    \end{subfigure}
        \begin{subfigure}{\figwidth}
    \includegraphics[width=1\linewidth]{figures_results/book_SNR_20_repeat_ind_1_image.png}
    \caption*{7.07dB}
    \includegraphics[width=1\linewidth]{figures_results/book_SNR_20_repeat_ind_1_depth.png}
        \caption*{41.97mm} 
    \end{subfigure}
        \begin{subfigure}{\figwidth}
    \includegraphics[width=1\linewidth]{figures_results/book_SNR_30_repeat_ind_1_image.png}
    \caption*{17.24dB}
    \includegraphics[width=1\linewidth]{figures_results/book_SNR_30_repeat_ind_1_depth.png}
        \caption*{21.11mm} 
    \end{subfigure}
        \begin{subfigure}{\figwidth}
    \includegraphics[width=1\linewidth]{figures_results/book_SNR_40_repeat_ind_1_image.png}
    \caption*{26.17dB}
    \includegraphics[width=1\linewidth]{figures_results/book_SNR_40_repeat_ind_1_depth.png}
        \caption*{19.42mm} 
    \end{subfigure}
    
             \begin{subfigure}{\figwidth}
    %  \caption*{Original}
    \includegraphics[width=1\linewidth]{figures_results/cones_scene_image.png}
         \caption*{PSNR:}
    \includegraphics[width=1\linewidth]{figures_results/cones_scene_depth.png}
        \caption*{RMSE:}
    \end{subfigure}
        \begin{subfigure}{\figwidth}
        % \caption*{20dB}
    \includegraphics[width=1\linewidth]{figures_results/cones_SNR_20_repeat_ind_1_image.png}
     \caption*{3.22dB}
    \includegraphics[width=1\linewidth]{figures_results/cones_SNR_20_repeat_ind_1_depth.png}
        \caption*{120.66mm} 
    \end{subfigure}
        \begin{subfigure}{\figwidth}
        % \caption*{30dB}
    \includegraphics[width=1\linewidth]{figures_results/cones_SNR_30_repeat_ind_1_image.png}
     \caption*{13.76dB}
    \includegraphics[width=1\linewidth]{figures_results/cones_SNR_30_repeat_ind_1_depth.png}
        \caption*{43.52mm} 
    \end{subfigure}
        \begin{subfigure}{\figwidth}
        % \caption*{40dB}
    \includegraphics[width=1\linewidth]{figures_results/cones_SNR_40_repeat_ind_1_image.png}
     \caption*{23.70dB}
    \includegraphics[width=1\linewidth]{figures_results/cones_SNR_40_repeat_ind_1_depth.png}
        \caption*{29.22mm} 
    \end{subfigure}
    ~~~
        \begin{subfigure}{\figwidth}
    \includegraphics[width=1\linewidth]{figures_results/corner_scene_image.png}
    \caption*{PSNR:}
    \includegraphics[width=1\linewidth]{figures_results/corner_scene_depth.png}
    \caption*{RMSE:}
    \end{subfigure}
    \begin{subfigure}{\figwidth}
    \includegraphics[width=1\linewidth]{figures_results/corner_SNR_20_repeat_ind_1_image.png}
    \caption*{6.33dB}
    \includegraphics[width=1\linewidth]{figures_results/corner_SNR_20_repeat_ind_1_depth.png}
        \caption*{32810.73mm} 
    \end{subfigure}
    \begin{subfigure}{\figwidth}
    \includegraphics[width=1\linewidth]{figures_results/corner_SNR_30_repeat_ind_1_image.png}
    \caption*{16.52dB}
    \includegraphics[width=1\linewidth]{figures_results/corner_SNR_30_repeat_ind_1_depth.png}
        \caption*{420.07mm} 
    \end{subfigure}
        \begin{subfigure}{\figwidth}
    \includegraphics[width=1\linewidth]{figures_results/corner_SNR_40_repeat_ind_1_image.png}
    \caption*{26.32dB}
    \includegraphics[width=1\linewidth]{figures_results/corner_SNR_40_repeat_ind_1_depth.png}
        \caption*{304.35mm} 
    \end{subfigure}
    
    \caption{Additional results for reconstruction from measurements at different levels of signal-to-noise ratio (SNR). The sequence in top left is for \textit{Whiteboard}, top right is \textit{Playroom}, middle left left \textit{Moebius}, middle right is \textit{Books}, bottom left is \textit{Cones}, and bottom right is \textit{Corner} dataset.}

    \label{fig:noise_examples_supp}
\end{figure*}

% SIZE OF SENSOR PIXELS

\begin{figure*}
    \centering
    \begin{subfigure}{\figwidth}
    \caption*{Original}
    \includegraphics[width=1\linewidth]{figures_results/whiteboard_scene_image.png}
    \caption*{Image PSNR:}
    \includegraphics[width=1\linewidth]{figures_results/whiteboard_scene_depth.png}
        \caption*{Depth RMSE:}
    \end{subfigure}
    \begin{subfigure}{\figwidth}
    \caption*{25$\mu$m} 
    \includegraphics[width=1\linewidth]{figures_results/whiteboard_pixel_size_25_image.png}
    \caption*{30.99dB}
    \includegraphics[width=1\linewidth]{figures_results/whiteboard_pixel_size_25_depth.png}
        \caption*{140.43mm} 
    \end{subfigure}
        \begin{subfigure}{\figwidth}
    \caption*{50$\mu$m} 
    \includegraphics[width=1\linewidth]{figures_results/whiteboard_pixel_size_50_image.png}
    \caption*{28.64dB}
    \includegraphics[width=1\linewidth]{figures_results/whiteboard_pixel_size_50_depth.png}
        \caption*{128.72mm} 
    \end{subfigure}
        \begin{subfigure}{\figwidth}
    \caption*{100$\mu$m} 
    \includegraphics[width=1\linewidth]{figures_results/whiteboard_pixel_size_100_image.png}
    \caption*{26.17dB}
    \includegraphics[width=1\linewidth]{figures_results/whiteboard_pixel_size_100_depth.png}
        \caption*{159.13mm} 
    \end{subfigure}
    ~~~
        \begin{subfigure}{\figwidth}
            \caption*{Original}
    \includegraphics[width=1\linewidth]{figures_results/playroom_scene_image.png}
    \caption*{Image PSNR:}
    \includegraphics[width=1\linewidth]{figures_results/playroom_scene_depth.png}
        \caption*{Depth RMSE:}
    \end{subfigure}
    \begin{subfigure}{\figwidth}
        \caption*{25$\mu$m} 
    \includegraphics[width=1\linewidth]{figures_results/playroom_pixel_size_25_image.png}
    \caption*{33.95dB}
    \includegraphics[width=1\linewidth]{figures_results/playroom_pixel_size_25_depth.png}
        \caption*{167.15mm} 
    \end{subfigure}
        \begin{subfigure}{\figwidth}
            \caption*{50$\mu$m} 
    \includegraphics[width=1\linewidth]{figures_results/playroom_pixel_size_50_image.png}
    \caption*{32.99dB}
    \includegraphics[width=1\linewidth]{figures_results/playroom_pixel_size_50_depth.png}
        \caption*{129.04mm} 
    \end{subfigure}
        \begin{subfigure}{\figwidth}
        \caption*{100$\mu$m} 
    \includegraphics[width=1\linewidth]{figures_results/playroom_pixel_size_100_image.png}
    \caption*{30.58dB}
    \includegraphics[width=1\linewidth]{figures_results/playroom_pixel_size_100_depth.png}
        \caption*{109.12mm} 
    \end{subfigure}
    
        \begin{subfigure}{\figwidth}
    \includegraphics[width=1\linewidth]{figures_results/moebius_scene_image.png}
    \caption*{Image PSNR:}
    \includegraphics[width=1\linewidth]{figures_results/moebius_scene_depth.png}
        \caption*{Depth RMSE:}
    \end{subfigure}
    \begin{subfigure}{\figwidth}
    \includegraphics[width=1\linewidth]{figures_results/moebius_pixel_size_25_image.png}
    \caption*{32.12dB}
    \includegraphics[width=1\linewidth]{figures_results/moebius_pixel_size_25_depth.png}
        \caption*{22.42mm} 
    \end{subfigure}
        \begin{subfigure}{\figwidth}
    \includegraphics[width=1\linewidth]{figures_results/moebius_pixel_size_50_image.png}
    \caption*{29.64dB}
    \includegraphics[width=1\linewidth]{figures_results/moebius_pixel_size_50_depth.png}
        \caption*{16.19mm} 
    \end{subfigure}
        \begin{subfigure}{\figwidth}
    \includegraphics[width=1\linewidth]{figures_results/moebius_pixel_size_100_image.png}
    \caption*{27.18dB}
    \includegraphics[width=1\linewidth]{figures_results/moebius_pixel_size_100_depth.png}
        \caption*{14.14mm} 
    \end{subfigure}
    ~~~
            \begin{subfigure}{\figwidth}
    \includegraphics[width=1\linewidth]{figures_results/book_scene_image.png}
    \caption*{Image PSNR:}
    \includegraphics[width=1\linewidth]{figures_results/book_scene_depth.png}
        \caption*{Depth RMSE:}
    \end{subfigure}
    \begin{subfigure}{\figwidth}
    \includegraphics[width=1\linewidth]{figures_results/book_pixel_size_25_image.png}
    \caption*{33.04dB}
    \includegraphics[width=1\linewidth]{figures_results/book_pixel_size_25_depth.png}
        \caption*{23.82mm} 
    \end{subfigure}
        \begin{subfigure}{\figwidth}
    \includegraphics[width=1\linewidth]{figures_results/book_pixel_size_50_image.png}
    \caption*{31.14dB}
    \includegraphics[width=1\linewidth]{figures_results/book_pixel_size_50_depth.png}
        \caption*{19.72mm} 
    \end{subfigure}
        \begin{subfigure}{\figwidth}
    \includegraphics[width=1\linewidth]{figures_results/book_pixel_size_100_image.png}
    \caption*{28.40dB}
    \includegraphics[width=1\linewidth]{figures_results/book_pixel_size_100_depth.png}
        \caption*{19.40 mm} 
    \end{subfigure}
    
    \begin{subfigure}{\figwidth}
    %  \caption*{Original}
    \includegraphics[width=1\linewidth]{figures_results/cones_scene_image.png}
    \caption*{Image PSNR:}
    \includegraphics[width=1\linewidth]{figures_results/cones_scene_depth.png}
        \caption*{Depth RMSE:}
    \end{subfigure}
    \begin{subfigure}{\figwidth}
    %  \caption*{25$\mu$m}
    \includegraphics[width=1\linewidth]{figures_results/cones_pixel_size_25_image.png}
    \caption*{33.90dB}
    \includegraphics[width=1\linewidth]{figures_results/cones_pixel_size_25_depth.png}
        \caption*{39.64mm} 
    \end{subfigure}
        \begin{subfigure}{\figwidth}
        %  \caption*{50$\mu$m}
    \includegraphics[width=1\linewidth]{figures_results/cones_pixel_size_50_image.png}
    \caption*{32.83dB}
    \includegraphics[width=1\linewidth]{figures_results/cones_pixel_size_50_depth.png}
        \caption*{28.70mm} 
    \end{subfigure}
        \begin{subfigure}{\figwidth}
        %  \caption*{100$\mu$m}
    \includegraphics[width=1\linewidth]{figures_results/cones_pixel_size_100_image.png}
    \caption*{31.22dB}
    \includegraphics[width=1\linewidth]{figures_results/cones_pixel_size_100_depth.png}
        \caption*{17.56mm} 
    \end{subfigure}
    ~~~
    \begin{subfigure}{\figwidth}
    \includegraphics[width=1\linewidth]{figures_results/corner_scene_image.png}
    \caption*{Image PSNR:}
    \includegraphics[width=1\linewidth]{figures_results/corner_scene_depth.png}
        \caption*{Depth RMSE:}
    \end{subfigure}
    \begin{subfigure}{\figwidth}
    \includegraphics[width=1\linewidth]{figures_results/corner_pixel_size_25_image.png}
    \caption*{35.60dB}
    \includegraphics[width=1\linewidth]{figures_results/corner_pixel_size_25_depth.png}
        \caption*{358.98mm} 
    \end{subfigure}
        \begin{subfigure}{\figwidth}
    \includegraphics[width=1\linewidth]{figures_results/corner_pixel_size_50_image.png}
    \caption*{34.15dB}
    \includegraphics[width=1\linewidth]{figures_results/corner_pixel_size_50_depth.png}
        \caption*{282.61mm} 
    \end{subfigure}
        \begin{subfigure}{\figwidth}
    \includegraphics[width=1\linewidth]{figures_results/corner_pixel_size_100_image.png}
    \caption*{30.74dB}
    \includegraphics[width=1\linewidth]{figures_results/corner_pixel_size_100_depth.png}
        \caption*{267.94mm} 
    \end{subfigure}       

    \caption{Additional results for reconstruction from measurements with different sizes of pixels. The number of sensor pixels is fixed as $512\times512$. } 
    \label{fig:size_of_pixels_example_supp}
\end{figure*}

% METHODS COMPARISON

\begin{figure*}
    \centering
    \begin{subfigure}{\figwidth}
    \caption*{Original}
    \includegraphics[width=1\linewidth]{figures_results/whiteboard_scene_image.png}
    \caption*{Image PSNR:}
    \includegraphics[width=1\linewidth]{figures_results/whiteboard_scene_depth.png}
        \caption*{Depth RMSE:}
    \end{subfigure}
    \begin{subfigure}{\figwidth}
    \caption*{3D Grid \cite{antipa2018diffusercam}} 
    \includegraphics[width=1\linewidth]{figures_results/whiteboard_method_3d_grid_ndepth_30_image.png}
    \caption*{7.67dB}
    \includegraphics[width=1\linewidth]{figures_results/whiteboard_method_3d_grid_ndepth_30_depth.png}
        \caption*{437.46mm} 
    \end{subfigure}
        \begin{subfigure}{\figwidth}
    \caption*{Greedy \cite{asif2017lensless3D}} 
    \includegraphics[width=1\linewidth]{figures_results/whiteboard_method_greedy_ndepth_30_image.png}
    \caption*{15.31dB}
    \includegraphics[width=1\linewidth]{figures_results/whiteboard_method_greedy_ndepth_30_depth.png}
        \caption*{316.33mm} 
    \end{subfigure}
        \begin{subfigure}{\figwidth}
    \caption*{Ours} 
    \includegraphics[width=1\linewidth]{figures_results/whiteboard_pixel_size_50_image.png}
    \caption*{28.64dB}
    \includegraphics[width=1\linewidth]{figures_results/whiteboard_pixel_size_50_depth.png}
        \caption*{128.72mm} 
    \end{subfigure}
    ~~~
         \begin{subfigure}{\figwidth}
             \caption*{Original}
    \includegraphics[width=1\linewidth]{figures_results/playroom_scene_image.png}
    \caption*{Image PSNR:}
    \includegraphics[width=1\linewidth]{figures_results/playroom_scene_depth.png}
        \caption*{Depth RMSE:}
    \end{subfigure}
    \begin{subfigure}{\figwidth}
        \caption*{3D Grid \cite{antipa2018diffusercam}} 
    \includegraphics[width=1\linewidth]{figures_results/playroom_method_3d_grid_ndepth_30_image.png}
    \caption*{10.28dB}
    \includegraphics[width=1\linewidth]{figures_results/playroom_method_3d_grid_ndepth_30_depth.png}
        \caption*{359.62mm} 
    \end{subfigure}
        \begin{subfigure}{\figwidth}
            \caption*{Greedy \cite{asif2017lensless3D}} 
    \includegraphics[width=1\linewidth]{figures_results/playroom_method_greedy_ndepth_30_image.png}
    \caption*{16.02dB}
    \includegraphics[width=1\linewidth]{figures_results/playroom_method_greedy_ndepth_30_depth.png}
        \caption*{282.86mm} 
    \end{subfigure}
        \begin{subfigure}{\figwidth}
            \caption*{Ours} 
    \includegraphics[width=1\linewidth]{figures_results/playroom_pixel_size_50_image.png}
    \caption*{32.99dB}
    \includegraphics[width=1\linewidth]{figures_results/playroom_pixel_size_50_depth.png}
        \caption*{129.04mm} 
    \end{subfigure}
    
            \begin{subfigure}{\figwidth}
    \includegraphics[width=1\linewidth]{figures_results/moebius_scene_image.png}
    \caption*{Image PSNR:}
    \includegraphics[width=1\linewidth]{figures_results/moebius_scene_depth.png}
        \caption*{Depth RMSE:}
    \end{subfigure}
    \begin{subfigure}{\figwidth}
    \includegraphics[width=1\linewidth]{figures_results/moebius_method_3d_grid_ndepth_30_image.png}
    \caption*{5.26dB}
    \includegraphics[width=1\linewidth]{figures_results/moebius_method_3d_grid_ndepth_30_depth.png}
        \caption*{72.91mm} 
    \end{subfigure}
        \begin{subfigure}{\figwidth}
    \includegraphics[width=1\linewidth]{figures_results/moebius_method_greedy_ndepth_30_image.png}
    \caption*{12.75dB}
    \includegraphics[width=1\linewidth]{figures_results/moebius_method_greedy_ndepth_30_depth.png}
        \caption*{72.02mm} 
    \end{subfigure}
        \begin{subfigure}{\figwidth}
    \includegraphics[width=1\linewidth]{figures_results/moebius_pixel_size_50_image.png}
    \caption*{29.64dB}
    \includegraphics[width=1\linewidth]{figures_results/moebius_pixel_size_50_depth.png}
        \caption*{16.19mm} 
    \end{subfigure}
    ~~~
    \centering
    \begin{subfigure}{\figwidth}
    \includegraphics[width=1\linewidth]{figures_results/book_scene_image.png}
    \caption*{Image PSNR:}
    \includegraphics[width=1\linewidth]{figures_results/book_scene_depth.png}
        \caption*{Depth RMSE:}
    \end{subfigure}
    \begin{subfigure}{\figwidth}
    \includegraphics[width=1\linewidth]{figures_results/book_method_3d_grid_ndepth_30_image.png}
    \caption*{9.58dB}
    \includegraphics[width=1\linewidth]{figures_results/book_method_3d_grid_ndepth_30_depth.png}
        \caption*{73.15mm} 
    \end{subfigure}
        \begin{subfigure}{\figwidth}
    \includegraphics[width=1\linewidth]{figures_results/book_method_greedy_ndepth_30_image.png}
    \caption*{16.93dB}
    \includegraphics[width=1\linewidth]{figures_results/book_method_greedy_ndepth_30_depth.png}
        \caption*{65.56mm} 
    \end{subfigure}
        \begin{subfigure}{\figwidth}
    \includegraphics[width=1\linewidth]{figures_results/book_pixel_size_50_image.png}
    \caption*{31.14dB}
    \includegraphics[width=1\linewidth]{figures_results/book_pixel_size_50_depth.png}
        \caption*{19.72mm} 
    \end{subfigure}

    \begin{subfigure}{\figwidth}
        % \caption*{Original}
    \includegraphics[width=1\linewidth]{figures_results/cones_scene_image.png}
    \caption*{Image PSNR:}
    \includegraphics[width=1\linewidth]{figures_results/cones_scene_depth.png}
        \caption*{Depth RMSE:}
    \end{subfigure}
    \begin{subfigure}{\figwidth}
    % \caption*{3D Grid\cite{antipa2018diffusercam}} 
    \includegraphics[width=1\linewidth]{figures_results/cones_method_3d_grid_ndepth_30_image.png}
    \caption*{8.46dB}
    \includegraphics[width=1\linewidth]{figures_results/cones_method_3d_grid_ndepth_30_depth.png}
        \caption*{96.08mm} 
    \end{subfigure}
        \begin{subfigure}{\figwidth}
        % \caption*{Greedy\cite{asif2017lensless3D}} 
    \includegraphics[width=1\linewidth]{figures_results/cones_method_greedy_ndepth_30_image.png}
    \caption*{14.13dB}
    \includegraphics[width=1\linewidth]{figures_results/cones_method_greedy_ndepth_30_depth.png}
        \caption*{109.47mm} 
    \end{subfigure}
        \begin{subfigure}{\figwidth}
        % \caption*{Ours} 
    \includegraphics[width=1\linewidth]{figures_results/cones_pixel_size_50_image.png}
    \caption*{32.83dB}
    \includegraphics[width=1\linewidth]{figures_results/cones_pixel_size_50_depth.png}
        \caption*{28.70mm} 
    \end{subfigure}
    ~~~
        \begin{subfigure}{\figwidth}
    \includegraphics[width=1\linewidth]{figures_results/corner_scene_image.png}
    \caption*{Image PSNR:}
    \includegraphics[width=1\linewidth]{figures_results/corner_scene_depth.png}
    \caption*{Depth RMSE:}
    \end{subfigure}
    \begin{subfigure}{\figwidth}
    \includegraphics[width=1\linewidth]{figures_results/corner_method_3d_grid_ndepth_30_image.png}
     \caption*{6.10dB}
    \includegraphics[width=1\linewidth]{figures_results/corner_method_3d_grid_ndepth_30_depth.png}
        \caption*{1423.17mm} 
    \end{subfigure}
        \begin{subfigure}{\figwidth}
    \includegraphics[width=1\linewidth]{figures_results/corner_method_greedy_ndepth_30_image.png}
     \caption*{18.15dB}
    \includegraphics[width=1\linewidth]{figures_results/corner_method_greedy_ndepth_30_depth.png}
        \caption*{1506.94mm} 
    \end{subfigure}
        \begin{subfigure}{\figwidth}
    \includegraphics[width=1\linewidth]{figures_results/corner_pixel_size_50_image.png}
     \caption*{30.47dB}
    \includegraphics[width=1\linewidth]{figures_results/corner_pixel_size_50_depth.png}
        \caption*{267.94mm} 
    \end{subfigure}

    \caption{Additional results for comparison of our method against existing 3D grid method from \cite{adams2017rice_depth, antipa2018diffusercam} and greedy method from \cite{asif2017lensless3D}.}
    \label{fig:methods_comparison_supp}
\end{figure*}
